# Supplementary material for: Displacive quantum critical point in superconducting hydrides: The case of H$_3$S
Source: arXiv:2602.00833 source file (2026-07-03)
Supplement: Supplementary file 1 [file supplement.pdf]

# Supplemental Material: Ferroelectric quantum critical point in superconducting hydrides: The case of $\text{H}_3\text{S}$

Marco Cherubini,<sup>1,\*</sup> Abhishek Raghav,<sup>1,2</sup> and Michele Casula<sup>1,†</sup>

<sup>1</sup>*Institut de Minéralogie, de Physique des Matériaux et de Cosmochimie, CNRS, Sorbonne Université, 4 Place Jussieu, Paris, 75005, France*

<sup>2</sup>*RIKEN Center for Emergent Matter Science, 2-1 Hirosawa, Wako-shi, Saitama 351-0198, Japan*

(Dated: January 31, 2026)

## METHODS

We carried out path integral molecular dynamics (PIMD) simulations at various temperatures,  $T = 50$  K, 100 K, 150 K, 200 K and 300 K, using 100, 48, 32, 24 and 16 beads, respectively. The number of beads  $L_\tau$  employed for each temperature guarantees the convergence of the PIMD kinetic energy [1], by keeping the imaginary time step  $\delta\tau = \beta/L_\tau$  constant over the temperature grid, with  $\beta = 1/(k_B T)$ . The nuclei are evolved in time using the PILE integrator [2] within the i-Pi package [3]. A time step of 0.4 fs and a Langevin thermostat relaxation time of 50 fs are used. For classical molecular dynamics (MD), we performed simulations at the same temperatures with an additional simulation at  $T = 25$  K. Unfortunately, lower temperatures could not be explored due to ergodicity-breaking issues. We used a classical Langevin dynamic thermostat [2] with the same time step and thermostat relaxation time as in the PIMD simulations. Quantum simulations are approximately 40 - 50 ps long, except for those near the ferroelectric transition, where longer correlation times require simulations of the order of 200 - 400 ps to converge. On the other hand, all the classical trajectories are at least 400 ps long, thanks to their reduced computational cost. In principle, the  $\text{Im}\bar{3}\text{m} \rightarrow \text{R}\bar{3}\text{m}$  transformation is also accompanied by a trigonal distortion of the lattice. However, density functional theory (DFT) calculations [4] report a very weak trigonal distortion ( $\leq 0.05^\circ$ ), confirmed by our *ab initio* calculations. Supported by this finding, we run PIMD-NVT simulations constraining the unit cell vectors to the  $\text{Im}\bar{3}\text{m}$  shape, and letting the sulfur (S) and hydrogen (H) atoms free to move in the supercell. The corresponding pressure with the quantum contribution included is directly provided by the i-PI engine.

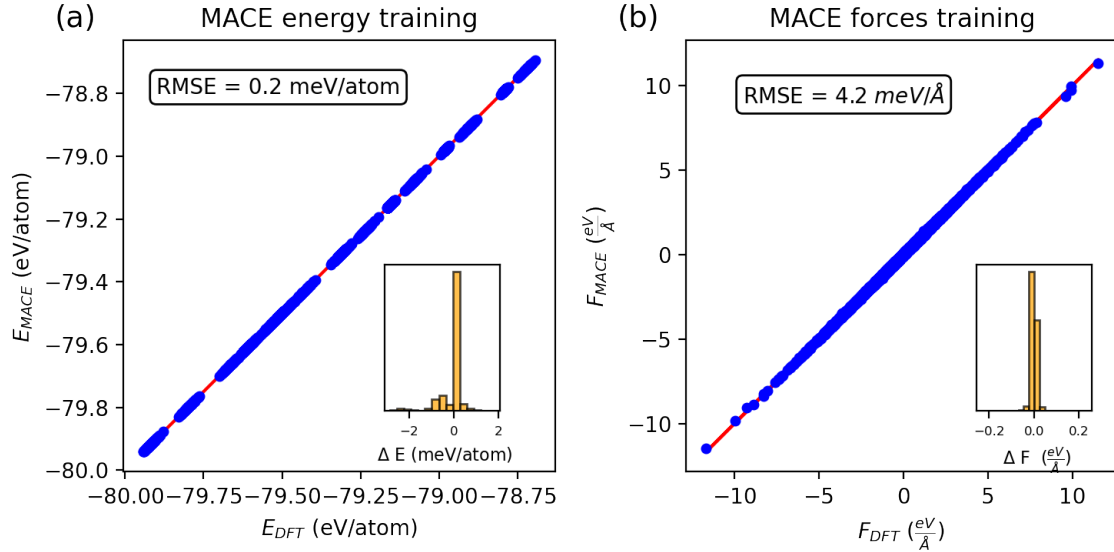

Figure 1. Evaluation of the MLIP on a 3660 configuration test set. Panel (a): Comparison between the energies predicted by the MACE model  $E_{\text{MACE}}$  and the DFT-BLYP reference energies  $E_{\text{DFT}}$ . Panel (b): forces predicted by the MACE model  $F_{\text{MACE}}$  compared with the DFT-BLYP references  $F_{\text{DFT}}$ . In both panels, the red line indicates the perfect correspondence. The histograms in the insets both panels show the corresponding error distributions.

*Ab initio* calculations of the forces in large supercells are extremely expensive, particularly at lower temperatures, where a large number of beads is required for convergence. To overcome this limitation, we trained a machine learning

interatomic potential (MLIP) exploiting *ab initio* PIMD and MD trajectories generated by some of us in a previous work [1]. In that case, the electronic part was solved within the Becke-Lee-Yang-Parr (BLYP) [5, 6] parametrization of the DFT exchange-correlation functional, as implemented in the Quantum Espresso package [7, 8]. The plain wave cut-off for the energy and for the charge density are set to 90 Ry and 420 Ry, respectively. A  $9 \times 9 \times 9$  reciprocal-space mesh was adopted with a Gaussian Fermi smearing of 0.03 Ry. For training, we used 14640 configurations that span a wide pressure range, from 40 GPa to 220 GPa at both  $T = 100$  K and  $T = 200$  K. Evenly distributed in pressure, about 35 % of them are randomly extracted from PIMD trajectories, the remaining ones are from classical MD. To train the model, we used MACE [9, 10], an equivariant message passing neural network [11, 12] that uses higher-body order messages, resulting in a fast and highly parallelizable model. We used a cutoff radius of 4.0 Å. We tested the performance of the trained MLIP on a test set containing 3660 configuration. In Figs. 1(a) and 1(b), we show the comparison between the predicted and reference energies and forces, respectively. The error distribution is plotted in the insets of the Figures, showing that errors are very small and centered around zero. The resulting mean absolute errors for the energies and forces are 0.363 meV/atom, and 5.25 meV/Å, respectively.

### FINITE-SIZE SCALING OF THE FERROELECTRIC TRANSITION LINE

In our PIMD simulations, we considered cells containing 32, 108 and 256 atoms corresponding to  $2 \times 2 \times 2$ ,  $3 \times 3 \times 3$  and  $4 \times 4 \times 4$  replicas of the primitive cell, respectively, with periodic boundary conditions. Computing different supercell sizes  $L \times L \times L$  allows us to extrapolate the ferroelectric transition pressure  $p_{\text{QCP}}(L, T)$  for each simulated temperature  $T$ . According to the 4D Ising universality class, the finite-size scaling of the critical coupling is given by[13–15]:

$$p_{\text{QCP}}(L, T) = p_{\text{QCP}}(\infty, T) + \alpha(T)L^{-2} \ln(L)^{-1/6}, \quad (1)$$

at fixed temperature  $T$ . The points  $p_{\text{QCP}}(L, T)$  are plotted in Fig. 2 as a function of  $1/L$  for all the simulated temperatures. The fits based on the functional form in Eq. 1 are also shown. To improve the precision of the fit, we assumed a linear temperature relation of the  $\alpha$  parameter in Eq. 1, such that  $\alpha(T) = \alpha_0 + \alpha_1 T$ . This has been empirically verified from our datapoints taken at  $T = 50$  K, 100 K, 150 K, where the critical pressure for the smallest system  $L = 2$  still falls in the range of validity of the MACE potential. With this model, the reduced  $\chi^2$  of our fits fluctuates around 1. Thus, Eq. 1 captures very well the spatial dependence of the critical couplings. It is another evidence of the validity of the 4D Ising universality class.

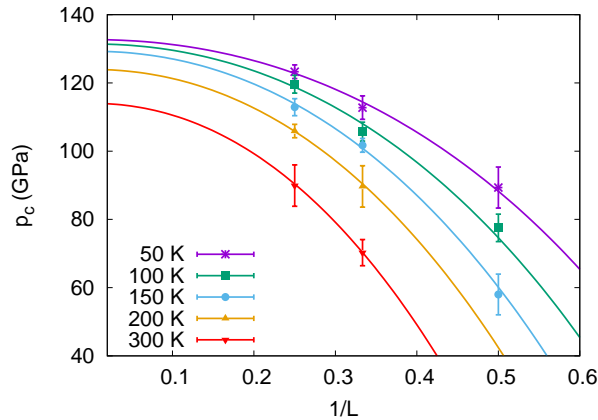

Figure 2. Ferroelectric critical pressures as a function of  $1/L$ , computed at different temperatures, as reported in the legend. The lines are the fitting functions, based on Eq. 1.

The ferroelectric transition line extrapolated to the thermodynamic limit ( $L = \infty$ ) is plotted in Fig. 3, together with the transition lines estimated from our simulations. The error bars on the extrapolated points are computed using the bootstrap method. The transition line for  $L = \infty$  as well the one for  $L = 4$  are also plotted in Fig. 1 of the main paper.

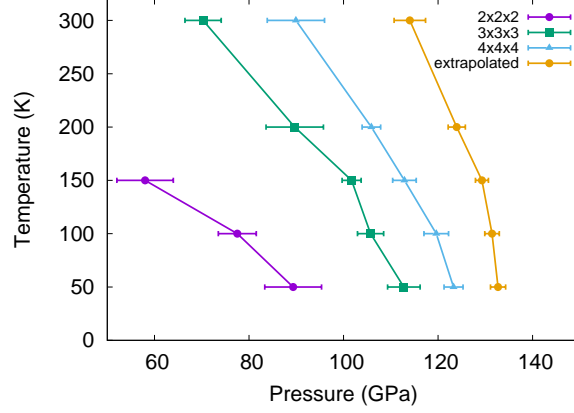

Figure 3. Ferroelectric transition lines computed at different sizes, as reported in the legend. The extrapolated values ( $L = \infty$ ) are obtained from the fit in Fig. 2.

### CLASSICAL FERROELECTRIC TRANSITION

The classical ferroelectric phase boundaries are computed using the same approach as for the quantum case, namely based on the evaluation of the local parameter and its fluctuations. For classical MD, we carried out simulations for  $L = 4$ , with the aim at performing a direct comparison with PIMD simulations at the same size, the largest attempted in PIMD. The simulation parameters of our classical MD runs are reported in the Methods Section. In Fig. 4(a), we report here the real and absolute value of the order parameter for all the temperatures investigated. As for the quantum case, we locate the ferroelectric transition at the pressure corresponding to the merging of the real and absolute values of the order parameter. In the classical situation, only thermal fluctuations are at play. If they are not strong enough, the protons cannot cross the potential barrier and remain frozen in one of the potential wells, resulting also in a drop of the variance of the order parameter (Fig. 4(b)).

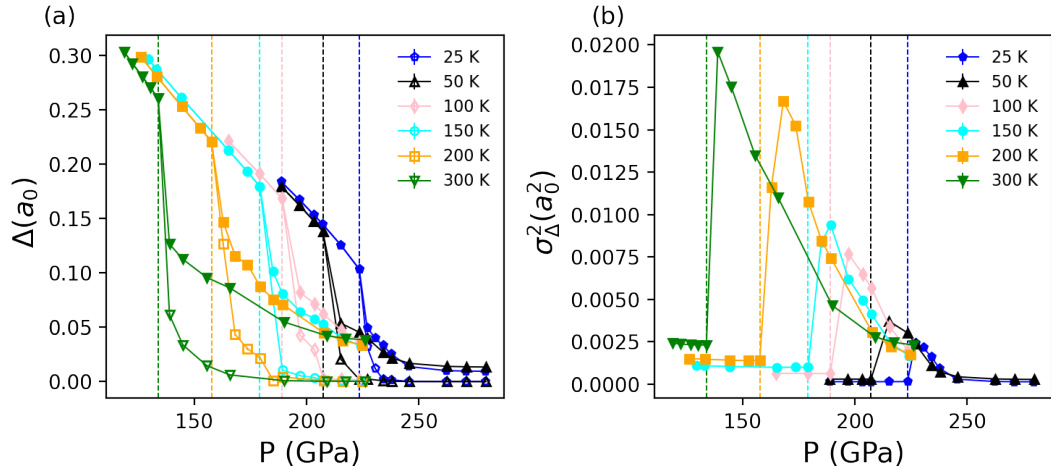

Figure 4. Panel (a): Order parameter for the classical ferroelectric transition. Full and empty symbols indicate the absolute and the real values of the order parameters, respectively. Different temperatures are reported: 25K in blue pentagons, 50K in black triangles, 100K in pink diamonds, 150K in cyan circles, 200K in orange squares and 300K in green reversed triangles. The vertical dashed lines indicate the transition pressures. Panel(b): Variance of the real value of the order parameter of panel (a). Colors and symbols retain the same meaning.

# PROTON DISTRIBUTIONS FROM PIMD AND CLASSICAL MD SIMULATIONS

In Eq. 2 of the main text, we define the local proton displacement, and in Fig. 2(c) of the main paper we plot its distribution along the S-S axis, expressed in crystal units, computed for  $L = 4$  at  $T = 50$  K. Here, we show the distributions of the proton local displacement as computed by PIMD for the same system size at higher temperatures, plotted in Fig. 5. In Fig. 6, we show also the classical distributions, computed by MD for the thermodynamic conditions specified in the plots. Like in the quantum case, from Fig. 6 we can clearly identify the ferroelectric transition, where the unimodal proton distribution is displaced from the S-S midpoint, the unimodal-to-bimodal variation, where the proton distribution acquires a bimodal shape, and finally a unimodal distribution centered in between the S-S distance at even higher pressures.

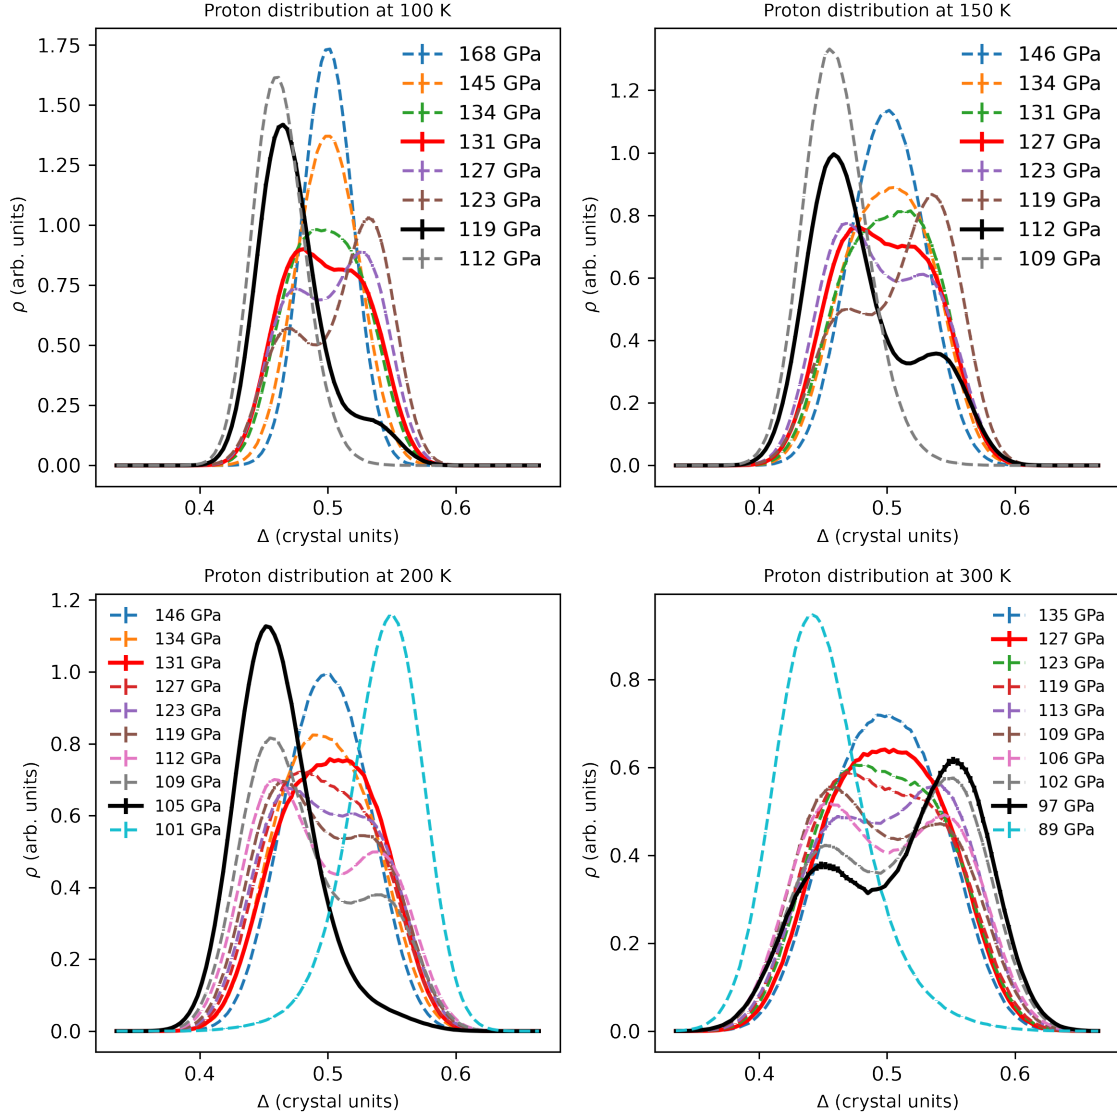

Figure 5. Proton centroid PIMD distributions along the S-S direction for several pressures at  $T = 100$  K, 150 K, 200 K and 300 K. The black and red thick curves correspond to the distributions at the ferroelectric transition and the unimodal-to-bimodal variation, respectively.

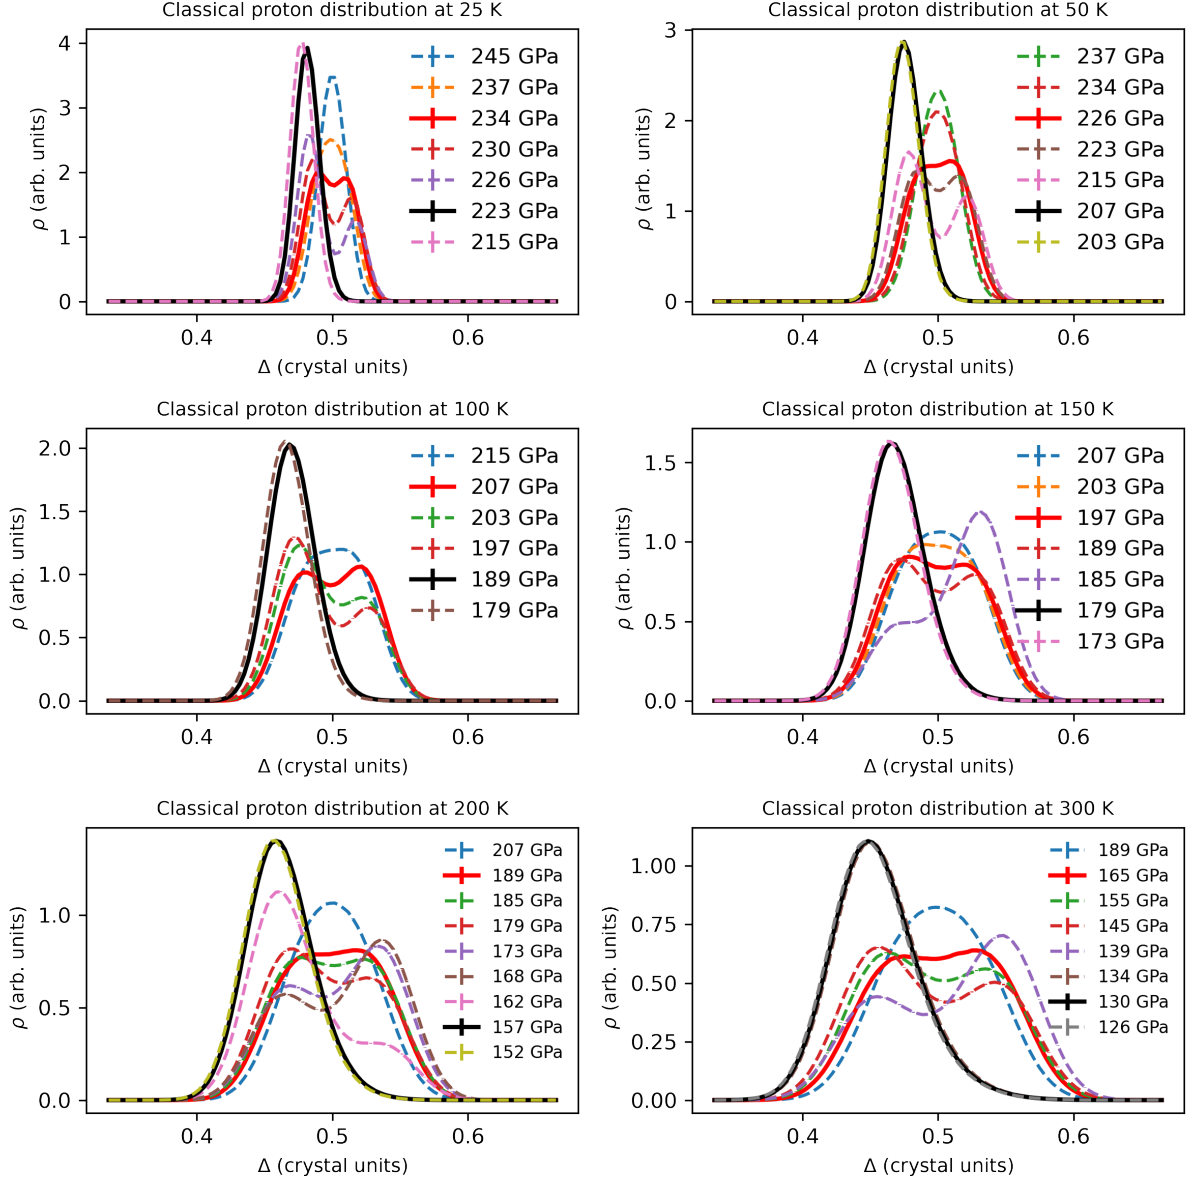

Figure 6. Classical proton MD distributions along the S-S direction for several pressures at  $T = 25$  K, 50 K, 100 K, 200 K and 300 K. The black and red thick curves correspond to the distributions at the ferroelectric transition and the unimodal-to-bimodal variation, respectively.

## QUANTUM AND CLASSICAL PHASE DIAGRAM

The classical ferroelectric phase boundaries are reported in Fig. 7 as well as in Fig. 1 of the main paper, together with the quantum transition line computed for  $L = 4$ . Compared to the quantum results, the classical ferroelectric transition is shifted to higher pressures. Moreover, the temperature dependence is stronger in the classical case, where there is an increase of about 57 % from room temperature to 50 K, larger than the 36 % increase found in the quantum regime for the same temperature range.

In Fig. 7, we also plot the  $(p, T)$  points where the centered unimodal proton distribution turns into a bimodal shape, signaling the formation of fluctuating local dipole moments, for both quantum and classical simulations. This information is extracted from Fig. 2(c) of the main paper and from Figs. 5 and 6 of the SM. In contrast to the quantum regime, where the unimodal-to-bimodal variation is only marginally affected by temperature, in the classical case we observe a strong temperature dependence. From room temperature down to 50 K, the unimodal-to-bimodal variation

pressure increases by about 40 %.

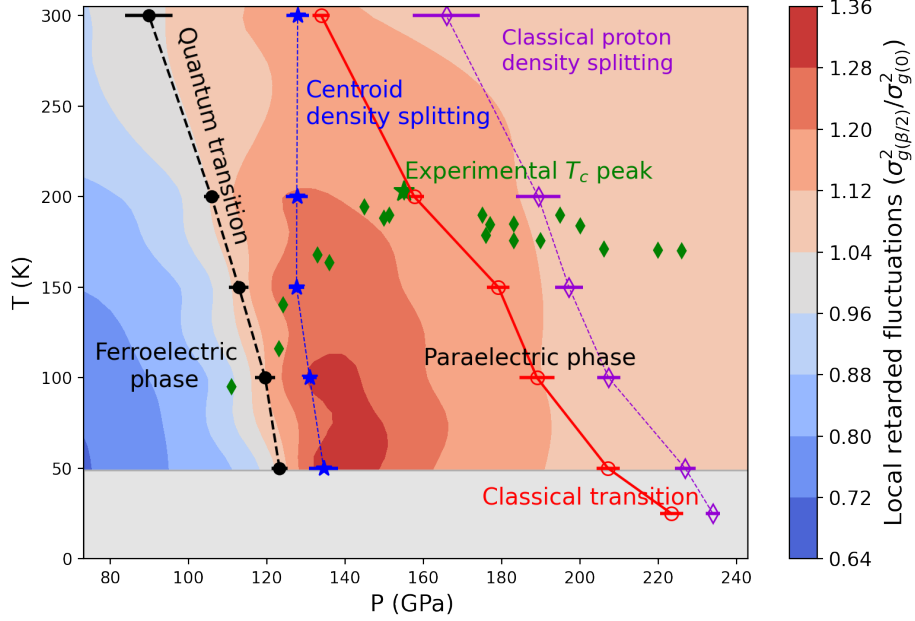

Figure 7. Quantum and classical phase diagram of sulfur hydride for  $L = 4$ . Filled black points and empty red points show the ferroelectric transition lines in quantum and classical simulations, respectively. Blue stars and violet empty diamonds indicate the unimodal-to-bimodal variation in the proton local displacement distribution (density splitting) from PIMD and MD simulations, respectively. Green diamonds are the experimental superconducting temperature, whose peak is shown by a green star[16, 17]. The colormap refers to the  $\sigma_{g(\beta/2)}^2/\sigma_{g(0)}^2$  ratio, as defined in the main text; it measures the relative intensity of the retarded fluctuations of local moments. In the dashed gray region, there is no data for interpolation, except for the classical case, where the lowest simulated temperature is 25 K.

## BEAD AND CENTROID RESOLVED QUANTUM ESTIMATORS

In Fig. 2 of the main paper as well as in Fig. 5, we reported the order parameter and its local distribution along the S-S direction for the centroid positions. It is useful to compare the results obtained when the bead resolution is taken into account and integrated over. In this case, we define the global displacement at the  $j$ -th PIMD iteration as

$$\Delta^{(j)} = \frac{1}{N_H L_\tau} \sum_{i=1}^{N_H} \sum_{k=1}^{L_\tau} [\tilde{r}_{H_i S_{i_1}}^{(j,k)} \cdot \hat{r}_{S_{i_1} S_{i_2}}^{(j,k)} - d_{S_{i_1} S_{i_2}}^{(j,k)} / 2], \quad (2)$$

where the  $r_{AB}^{(j,k)}$  vectors connect atom A and B at the  $j$ -th PIMD iteration and for  $k$ -th bead. In principle, the resulting global order parameter may differ from the one computed using the centroid positions. In fact, the projection in Eq. 2 over the versor pointing along the  $S_{i_1}$ - $S_{i_2}$  direction breaks the linear relationship between beads and centroids. To check for possible discrepancies, in Fig. 8 we compare the order parameter as function of pressure at 50 K using the centroid positions and the full bead resolution. It turns out that the choice between beads and centroids has a negligible effect on the estimates of the order parameter, for all pressures explored. The same situation is found for the other temperatures simulated.

While their averages are the same, the distributions differ between bead and centroid resolved estimators. This is apparent from Fig. 9, where we plot the local proton displacement distribution along the S-S direction at  $T = 50$  K and 200 K, to be compared with Fig. 2(c) of the main paper and Fig. 5 of this Supplemental Material (SM), respectively. The distributions computed on the bead positions are broader, owing to the quantum proton delocalization, better captured by the bead resolution. In the bead representation, the unimodal-to-bimodal variation is hidden by the appearance of a shoulder in the bead distribution, instead of a clear peak. Although this variation, and the corresponding local dipole moment formation, can always be detected by a higher-moment analysis of the bead distributions, it is much more transparent in the centroid distributions, which are indeed shown in the main paper.

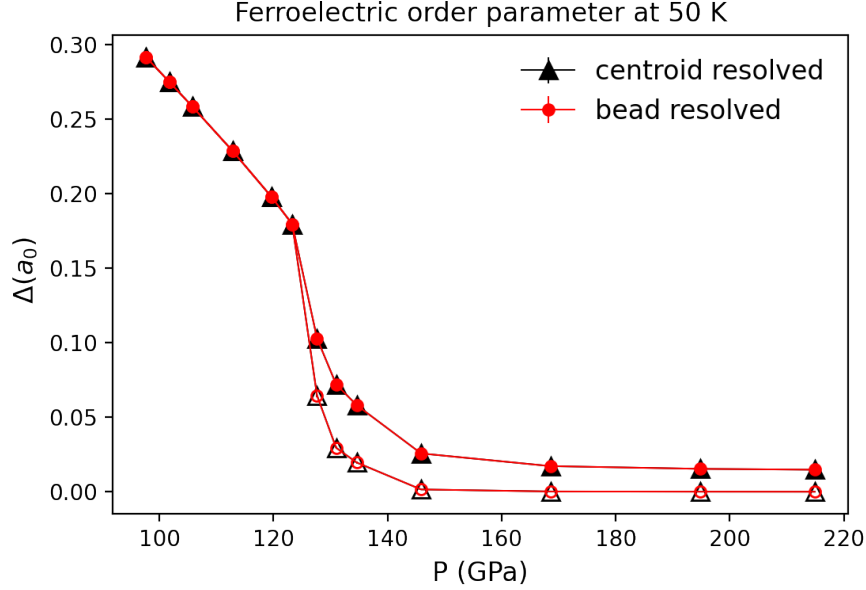

Figure 8. Order parameter at 50 K as a function of pressure. Full and empty symbols correspond to the real values of the order parameter  $\Delta$  and its absolute values  $\Delta_{\text{abs}}$ , respectively. Red (black) color is used to indicate values computed using the centroid positions (the full bead resolution).

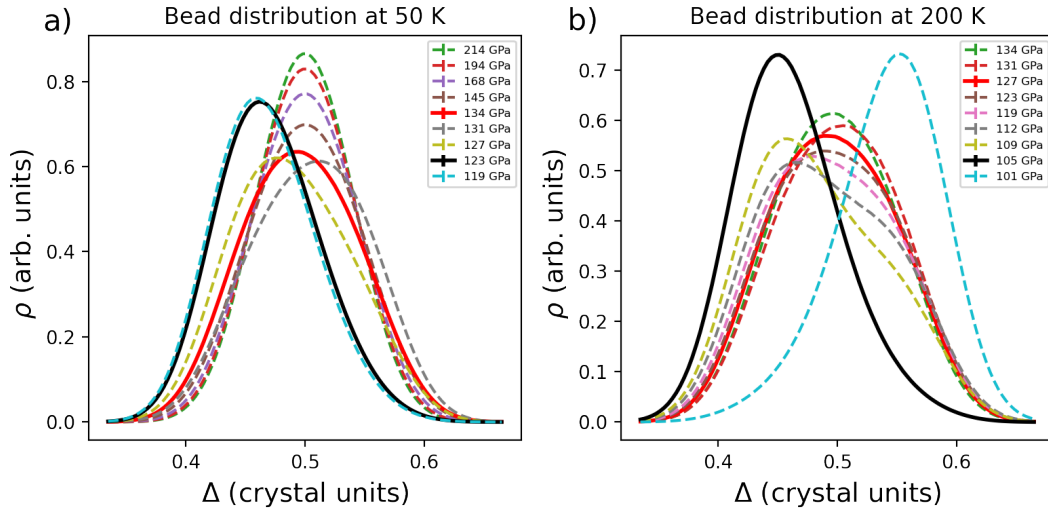

Figure 9. Proton bead distribution along the S-S direction for several pressures. PIMD simulations at 50 K and the 200 K are shown in panel (a) and (b), respectively. The thick red curve corresponds to the pressure where the proton centroid distribution (Fig. 2(c) of the main paper and Fig. 5 of the SM) becomes bimodal and the thick black one plots the distribution at the ferroelectric transition.

## PIMD PHONONS AND IMAGINARY-TIME RESOLVED PHONON GREEN FUNCTION

We evaluated anharmonic phonon frequencies at the PIMD level by computing the zero-frequency component of the Matsubara Green functions from the quantum displacement-displacement PIMD correlators using the method developed in Refs. [18, 19]. This method relies upon the calculation of the Kubo-transformed displacement-displacement correlators present in the definition of the imaginary-time phonon Green function:

$$G_{ij}(\tau, \mathbf{R}) = -\sqrt{m_i m_j} \langle T \delta x_i(\tau) \delta x_{j+\mathbf{R}}(0) \rangle, \quad (3)$$

where  $\delta x_i(\tau) = x_i(\tau) - \langle x_i \rangle$  are the atom displacements in the direction  $x$ , as defined in the main text. In Eq. 3,  $\{i, j\}$  run over the atomic indices of the unit cell, while  $\mathbf{R}$  is the index for a Bravais lattice vector contained in the simulation supercell. In PIMD, one can easily compute the imaginary-time averaged displacements  $\delta \tilde{x}_i = \int_0^\beta d\tau \delta x_i(\tau)/\beta$ , with  $\beta = 1/(k_B T)$  the inverse temperature. One can show that the Kubo-transformed phonon Green function  $\tilde{G}_{ij}(\mathbf{R}) = -\beta \sqrt{m_i m_j} \langle \delta \tilde{x}_i \delta \tilde{x}_{j+\mathbf{R}} \rangle$ , computed using the time averaged displacements, is the imaginary-time Fourier transform of Eq. 3 at zero Matsubara frequency ( $i\omega_0 = 0$ ), i.e. the static limit of the phonon Matsubara Green function. Furthermore, by relying on the translational invariance of the system, one can Fourier transform in space the Green function in Eq. 3, and get  $\tilde{G}_{ij}(\mathbf{q})$  on the supercell-allowed  $\mathbf{q}$  vectors. Thus,  $\tilde{G}_{ij}(\mathbf{q}) = G_{ij}(i\omega_0, \mathbf{q})$ . In other words,  $\tilde{\mathbf{G}}(\mathbf{q}) = -\frac{1}{\mathbf{D}(\mathbf{q})^{\text{harm}} + \mathbf{\Pi}(0, \mathbf{q})}$ , where  $\mathbf{D}^{\text{harm}}(\mathbf{q})$  represents the harmonic dynamical matrix of “bare” phonons at the wavevector  $\mathbf{q}$ , and  $\mathbf{\Pi}(0, \mathbf{q})$  is the static limit of the  $\mathbf{q}$ -dependent phonon self-energy  $\mathbf{\Pi}(i\omega_n, \mathbf{q})$ . Therefore, by computing the inverse  $\tilde{\mathbf{G}}^{-1}(\mathbf{q})$ , we have access to the squared phonon frequencies renormalized by static correlations. Indeed,  $\tilde{\mathbf{G}}^{-1}(\mathbf{q})$  enters the associated eigenvalue problem at each  $\mathbf{q}$ :

$$[\langle \delta \tilde{\mathbf{x}} \delta \tilde{\mathbf{x}}^T \rangle_{\mathbf{q}}^{-1}]_{ij} W_{jk}(\mathbf{q}) = m_i \beta \omega_k^2(\mathbf{q}) W_{ik}(\mathbf{q}), \quad (4)$$

where  $\omega_i^2(\mathbf{q})$  is the squared frequency of the  $i$ -th phonon mode at  $\mathbf{q}$ , and  $W_{ji}(\mathbf{q})$  is the eigenvectors matrix. In this work, we therefore solved Eq. 4 after sampling the necessary matrix elements by PIMD, in order to compute the anharmonic phonon branches. We evaluated them on a  $4 \times 4 \times 4$  grid, that has been interpolated to yield the anharmonic phonon dispersion plotted in Fig. 10 for different pressures across the ferromagnetic phase transition at  $T = 200$  K.

To study retardation effects of the one-body phonon Green function in Eq. 3, we also retained the full imaginary-time dependence of the displacement operators  $\delta x_i(\tau)$ , instead of replacing them by their time-averaged version  $\delta \tilde{x}_i$ . In practice, thanks to the imaginary-time periodicity of the phonon Green function, we computed a slightly modified version of Eq. 3, namely

$$G_{ij}(\tau, \mathbf{R}) = -\sqrt{m_i m_j} \langle \mathcal{T} \delta x_i(\tau + \tau') \delta x_{j+\mathbf{R}}(\tau') \rangle \quad \forall \tau', \quad (5)$$

in order to fully exploit the statistics coming from the PIMD samples at different imaginary-time slices. The explicit time dependence in Eq. 5 has been evaluated only for some selected cases, such as the Green function projected on the H local shuttling modes, as explained in the main paper. Indeed, bookkeeping the time dependence is heavier and much more memory demanding than just computing the Kubo-transformed time-integrated PIMD correlation functions.

## 2-BODY PHONON GREEN FUNCTION

Quantum fluctuations in proximity of the ferroelectric QCP manifest themselves not only in the one-body quantities but also in the two-body phonon Green functions. This is even more relevant in the context of “beyond-Migdal” theories of superconductivity, where the exchange of two-phonons is postulated in the electron-phonon coupling. In these theories, the integrated coupling depends on the strength of a local 2-body phonon Green function[20]. Therefore, it is interesting to study how the 2-body phonon Green function evolves across the ferroelectric transition.

As we have seen, PIMD gives access to the quantum imaginary time dynamics. Thus, we would like to study the imaginary-time dependent 2-body phonon Green function  $L(\tau, \tau')$ , defined as:

$$L(\tau, \tau') = \langle \mathcal{T} \delta x(\tau) \delta x(\tau') \delta x(0) \delta x(0) \rangle - \langle \mathcal{T} \delta x(\tau) \delta x(0) \rangle \langle \mathcal{T} \delta x(\tau') \delta x(0) \rangle, \quad (6)$$

where the quantum displacement-displacement correlator  $\langle \mathcal{T} \delta x(\tau) \delta x(0) \rangle$  is proportional to the one-body phonon Green function  $G(\tau)$  in Eqs. 3 and 5, with  $\delta x(\tau)$  the atomic displacement defined above. The 4-point correlators in Eq. 6 can be evaluated from the PIMD sampling as well as the 2-point correlators entering the definition of the one-body phonon Green function. Diagrammatically, Eq. 6 represents the connected, or correlated, part of the two-body phonon Green function, relevant in two-phonon coupling theories. We focus here on the equal-time 2-body phonon Green function, namely  $L_{\text{eq}}(\tau) \equiv L(\tau, \tau)$ , where  $\delta x(\tau)$  is taken for convenience as local proton displacements, defining the local dipole moments in  $\text{H}_3\text{S}$ . To measure the strength of this correlation across the ferroelectric transition, we compute the static limit of  $L_{\text{eq}}(i\omega_n)$ , with  $i\omega_n$  bosonic Matsubara frequencies. This corresponds to  $L_{\text{eq}}(i\omega_0) = \int_0^\beta d\tau L_{\text{eq}}(\tau)$ . We see that  $L_{\text{eq}}(i\omega_0)$  has a magnitude that progressively increases in the paraelectric phase as we move towards lower pressures, by reaching a peak at the ferroelectric transition, before rapidly decreasing at even lower pressures in the ferroelectric

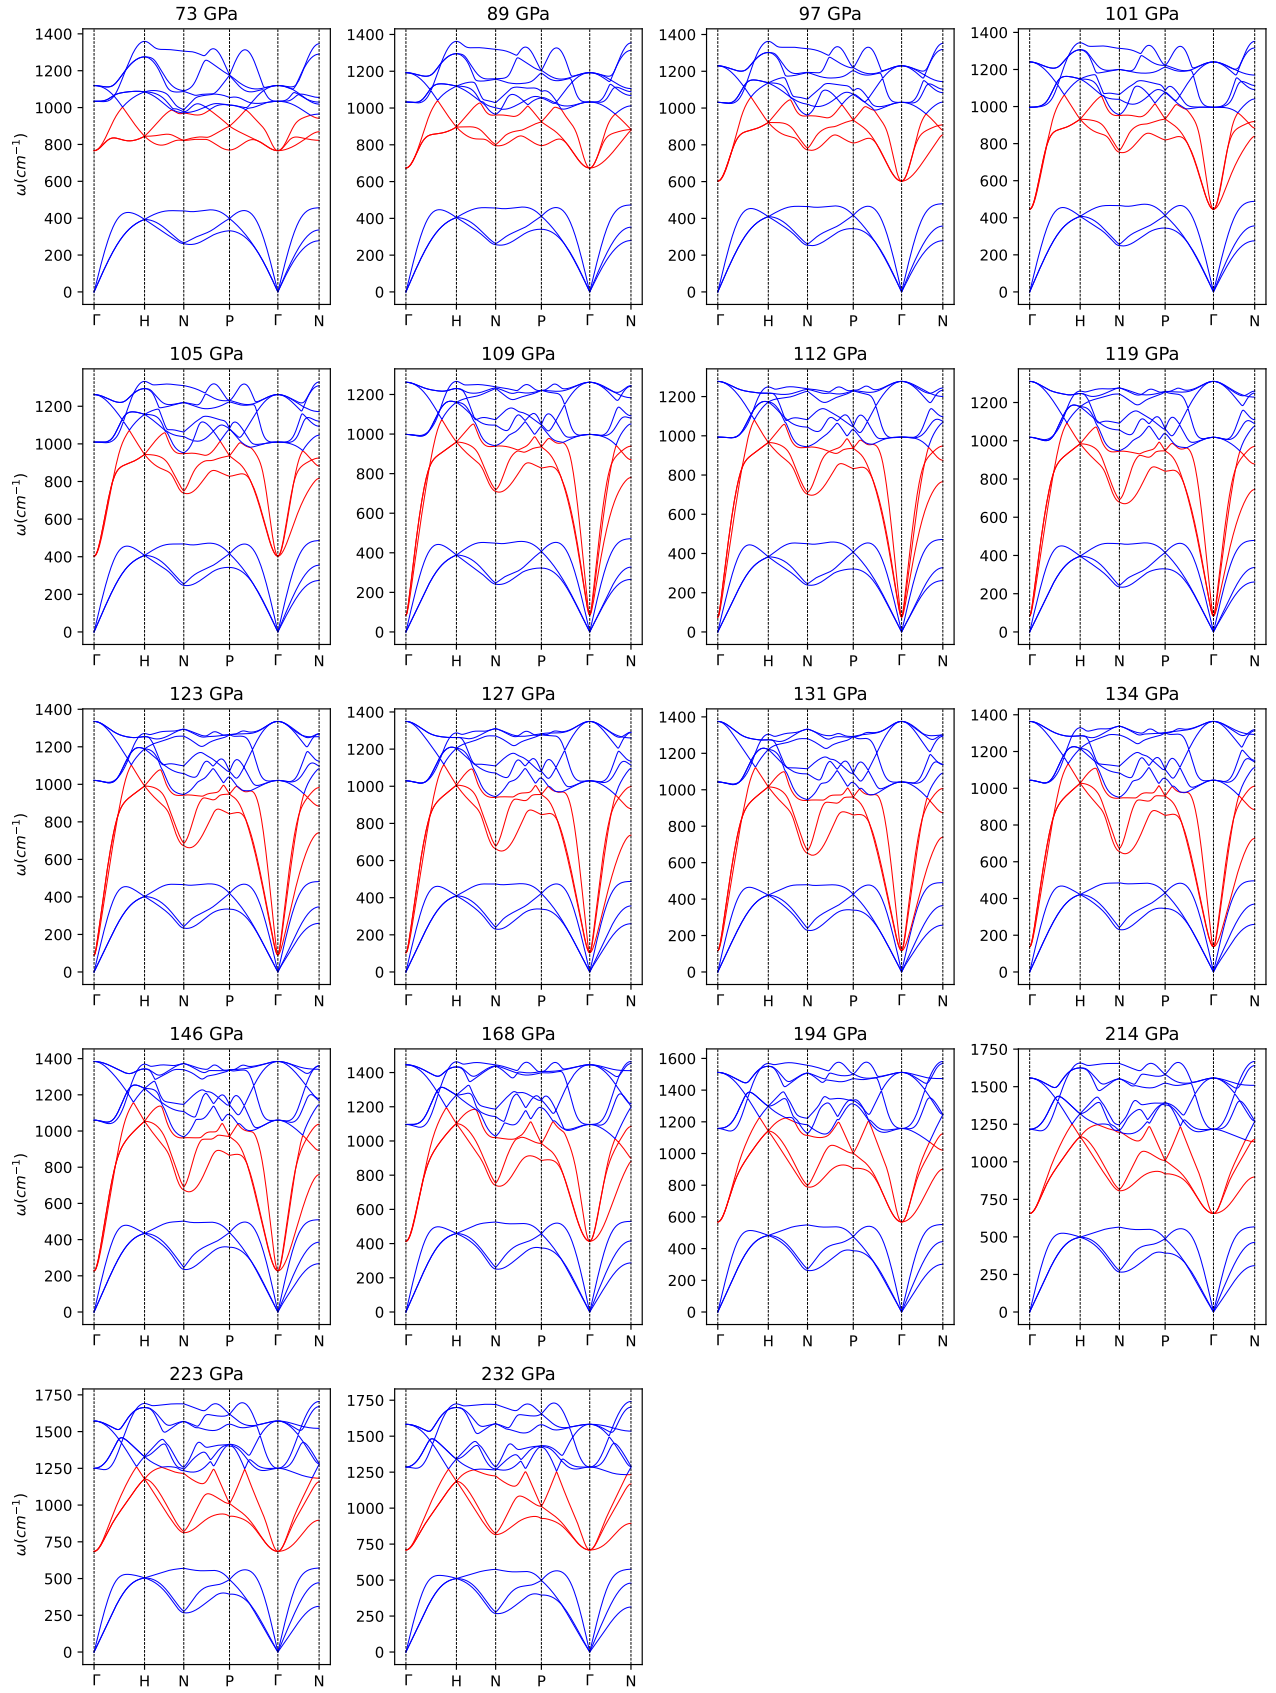

Figure 10. Anharmonic phonon dispersions computed by PIMD simulations at  $T = 200$  K performed in a  $4 \times 4 \times 4$  supercell ( $L = 4$ ), and then interpolated on a finer  $\mathbf{q}$  mesh. Before interpolation, the phonon frequencies  $\omega_i(\mathbf{q})$  and phonon patterns  $W_{ji}(\mathbf{q})$  have been computed by solving Eq. 4 on the supercell-allowed  $\mathbf{q}$  mesh. The branches that soften at the ferroelectric transition are highlighted in red color.

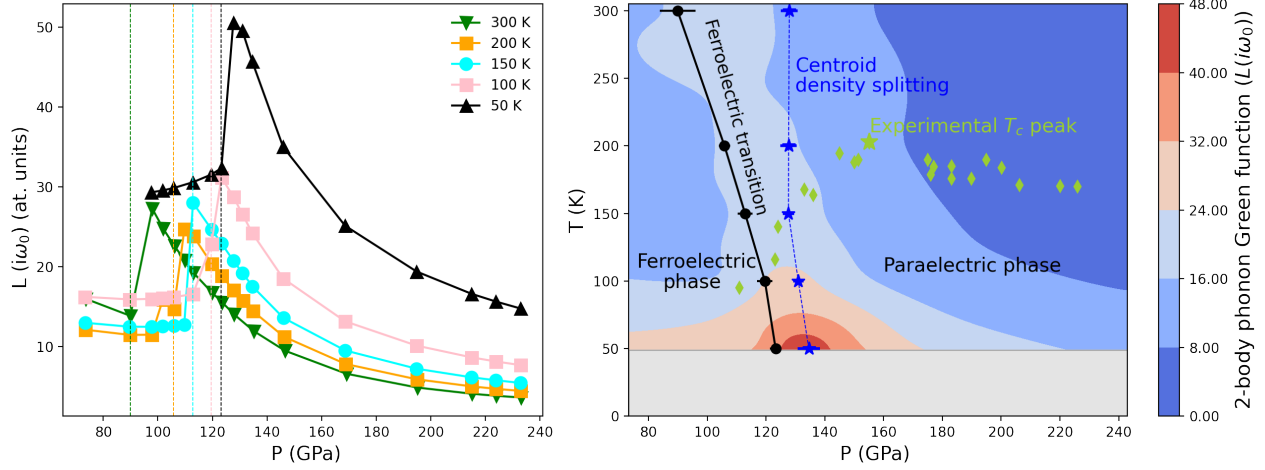

Figure 11. Static limit of the local 2-body phonon Green function  $L_{eq}(i\omega_0)$  computed by PIMD for  $L = 4$ , for the set of pressures and temperatures represented by the points in panel (a). The displacements in  $L_{eq}(i\omega_0)$  are the local proton displacements projected on the S-S axis, defining the local dipole moments. Panel (b): heatmap of  $L_{eq}(i\omega_0)$  in the  $(p, T)$  plane, obtained by a spline interpolation of the points in panel (a) via radially symmetric basis functions. The transition line and the centroid density splitting as determined for  $L = 4$ , together with the experimental  $T_c$  points[16, 17], are also plotted as reference.

phase. Thus, according to our calculations the two-phonon coupling channel could indeed be magnified close to the transition in the paraelectric side.

\* marco.cherubini@sorbonne-universite.fr

† michele.casula@sorbonne-universite.fr

- [1] R. Taureau, M. Cherubini, T. Morresi, and M. Casula, Quantum symmetrization transition in superconducting sulfur hydride from quantum Monte Carlo and path integral molecular dynamics, *npj Computational Materials* **10**, 10.1038/s41524-024-01239-0 (2024).
- [2] M. Ceriotti, M. Parrinello, T. E. Markland, and D. E. Manolopoulos, Efficient stochastic thermostating of path integral molecular dynamics, *The Journal of Chemical Physics* **133**, 10.1063/1.3489925 (2010).
- [3] M. Ceriotti, J. More, and D. E. Manolopoulos, i-PI: A Python interface for ab initio path integral molecular dynamics simulations, *Computer Physics Communications* **185**, 1019–1026 (2014).
- [4] R. Bianco, I. Errea, M. Calandra, and F. Mauri, High-pressure phase diagram of hydrogen and deuterium sulfides from first principles: Structural and vibrational properties including quantum and anharmonic effects, *Phys. Rev. B* **97**, 214101 (2018).
- [5] A. D. Becke, Density-functional exchange-energy approximation with correct asymptotic behavior, *Phys. Rev. A* **38**, 3098 (1988).
- [6] C. Lee, W. Yang, and R. G. Parr, Development of the Colle-Salvetti correlation-energy formula into a functional of the electron density, *Physical review B* **37**, 785 (1988).
- [7] P. Giannozzi, S. Baroni, N. Bonini, M. Calandra, R. Car, C. Cavazzoni, D. Ceresoli, G. L. Chiarotti, M. Cococcioni, I. Dabo, A. Dal Corso, S. de Gironcoli, S. Fabris, G. Fratesi, R. Gebauer, U. Gerstmann, C. Gougoussis, A. Kokalj, M. Lazzeri, L. Martin-Samos, N. Marzari, F. Mauri, R. Mazzarello, S. Paolini, A. Pasquarello, L. Paulatto, C. Sbraccia, S. Scandolo, G. Sclauzero, A. P. Seitsonen, A. Smogunov, P. Umari, and R. M. Wentzcovitch, QUANTUM ESPRESSO: a modular and open-source software project for quantum simulations of materials, *Journal of Physics: Condensed Matter* **21**, 395502 (2009).
- [8] P. Giannozzi, O. Andreussi, T. Brumme, O. Bunau, M. Buongiorno Nardelli, M. Calandra, R. Car, C. Cavazzoni, D. Ceresoli, M. Cococcioni, N. Colonna, I. Carnimeo, A. Dal Corso, S. de Gironcoli, P. Delugas, R. A. DiStasio, A. Ferretti, A. Floris, G. Fratesi, G. Fugallo, R. Gebauer, U. Gerstmann, F. Giustino, T. Gorni, J. Jia, M. Kawamura, H.-Y. Ko, A. Kokalj, E. Küçükbenli, M. Lazzeri, M. Marsili, N. Marzari, F. Mauri, N. L. Nguyen, H.-V. Nguyen, A. Otero-de-la Roza, L. Paulatto, S. Poncé, D. Rocca, R. Sabatini, B. Santra, M. Schlipf, A. P. Seitsonen, A. Smogunov, I. Timrov, T. Thonhauser, P. Umari, N. Vast, X. Wu, and S. Baroni, Advanced capabilities for materials modelling with Quantum ESPRESSO, *Journal of Physics: Condensed Matter* **29**, 465901 (2017).
- [9] I. Batatia, D. P. Kovacs, G. N. C. Simm, C. Ortner, and G. Csanyi, MACE: Higher Order Equivariant Message Passing Neural Networks for Fast and Accurate Force Fields, in *Advances in Neural Information Processing Systems*, edited by

- A. H. Oh, A. Agarwal, D. Belgrave, and K. Cho (2022).
- [10] I. Batatia, S. Batzner, D. P. Kovács, A. Musaelian, G. N. C. Simm, R. Drautz, C. Ortner, B. Kozinsky, and G. Csányi, The Design Space of E(3)-Equivariant Atom-Centered Interatomic Potentials (2022), arXiv:2205.06643.
  - [11] J. Gilmer, S. S. Schoenholz, P. F. Riley, O. Vinyals, and G. E. Dahl, Neural Message Passing for Quantum Chemistry, in *Proceedings of the 34th International Conference on Machine Learning*, Proceedings of Machine Learning Research, Vol. 70, edited by D. Precup and Y. W. Teh (PMLR, 2017) pp. 1263–1272.
  - [12] M. M. Bronstein, J. Bruna, T. Cohen, and P. Veličković, Geometric Deep Learning: Grids, Groups, Graphs, Geodesics, and Gauges (2021).
  - [13] E. Brézin, An investigation of finite size scaling, *Journal de Physique* **43**, 15 (1982).
  - [14] N. Aktekin, The finite-size scaling functions of the four-dimensional Ising model, *Journal of Statistical Physics* **104**, 1397 (2001).
  - [15] R. Kenna, Finite size scaling for  $O(N)$   $\varphi^4$ -theory at the upper critical dimension, *Nuclear Physics B* **691**, 292 (2004).
  - [16] A. P. Drozdov, M. I. Eremets, I. A. Troyan, V. Ksenofontov, and S. I. Shylin, Conventional superconductivity at 203 kelvin at high pressures in the sulfur hydride system, *Nature* **525**, 73 (2015).
  - [17] M. Einaga, M. Sakata, T. Ishikawa, K. Shimizu, M. I. Eremets, A. P. Drozdov, I. A. Troyan, N. Hirao, and Y. Ohishi, Crystal structure of the superconducting phase of sulfur hydride, *Nature Physics* **12**, 835 (2016).
  - [18] T. Morresi, L. Paulatto, R. Vuilleumier, and M. Casula, Probing anharmonic phonons by quantum correlators: A path integral approach, *The Journal of Chemical Physics* **154**, 224108 (2021).
  - [19] T. Morresi, R. Vuilleumier, and M. Casula, Hydrogen phase-IV characterization by full account of quantum anharmonicity, *Physical Review B* **106**, 054109 (2022).
  - [20] D. E. Kiselov and M. V. Feigel'man, Theory of superconductivity due to Ngai's mechanism in lightly doped  $\text{SrTiO}_3$ , *Physical Review B* **104**, 10.1103/physrevb.104.1220506 (2021).
